# Supplementary material for: Anisotropic optical properties of detwinned BaFe$_{2}$As$_{2}$
Source: arXiv:2006.16382 source file (2020-11-10)
Supplement: Supplementary file 1 [file supplemental.pdf]

# Supplementary material for "Anisotropic optical properties of detwinned $BaFe_2As_2$"

Christopher C. Homes,[1,*] Thomas Wolf,[2] and Christoph Meingast[2,†]

[1] *Condensed Matter Physics and Materials Science Division, Brookhaven National Laboratory, Upton, New York 11973, USA*

[2] *Institute for Quantum Materials and Technologies, Karlsruhe Institute of Technology, 76021 Karlsruhe, Germany*

(Dated: September 29, 2020)

## REFLECTIVITY

The temperature dependence of the reflectivity of a detwinned sample of $BaFe_2As_2$ ($T_N \simeq 138$ K) is shown over a wide frequency range for light polarized along the *a* and *b* axes in Figs. S1(a) and S1(b), respectively; the axes refer to the orthorhombic phase. The temperature dependent behavior of the reflectivity is restricted to energies below about 1 eV; above this energy there little temperature or polarization dependence. Overall, the spectra are qualitatively similar to those of Nakajima *et al.* [1].

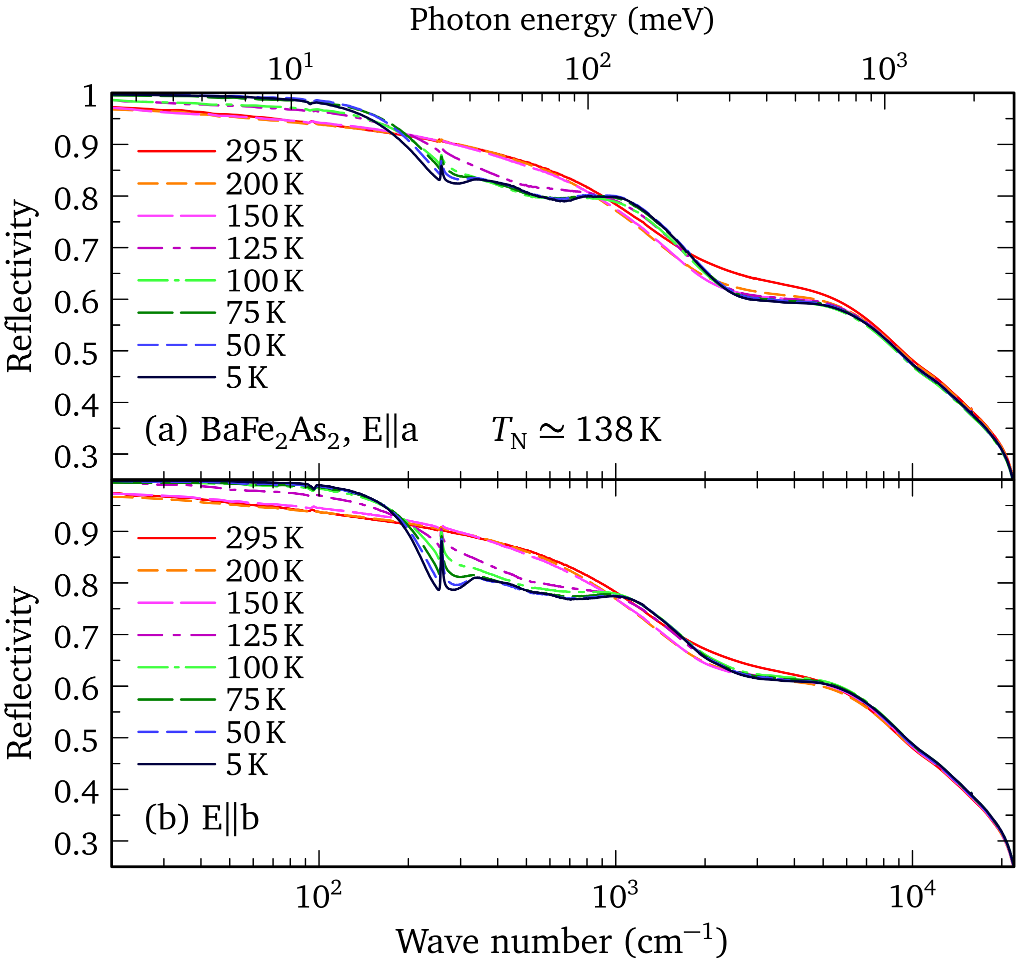


Figure S1. The temperature dependence of the reflectivity versus the log of the frequency of a detwinned sample of $BaFe_2As_2$ for light polarized along the: (a) *a* axis; (b) *b* axis.

## OPTICAL CONDUCTIVITY

The temperature dependence of the real part of the optical conductivity determined from a Kramers-Kronig analysis of the reflectivity is shown over a wide range for light polarized along the $a$ and $b$ axes in Figs. S2(a) and S2(b), respectively.

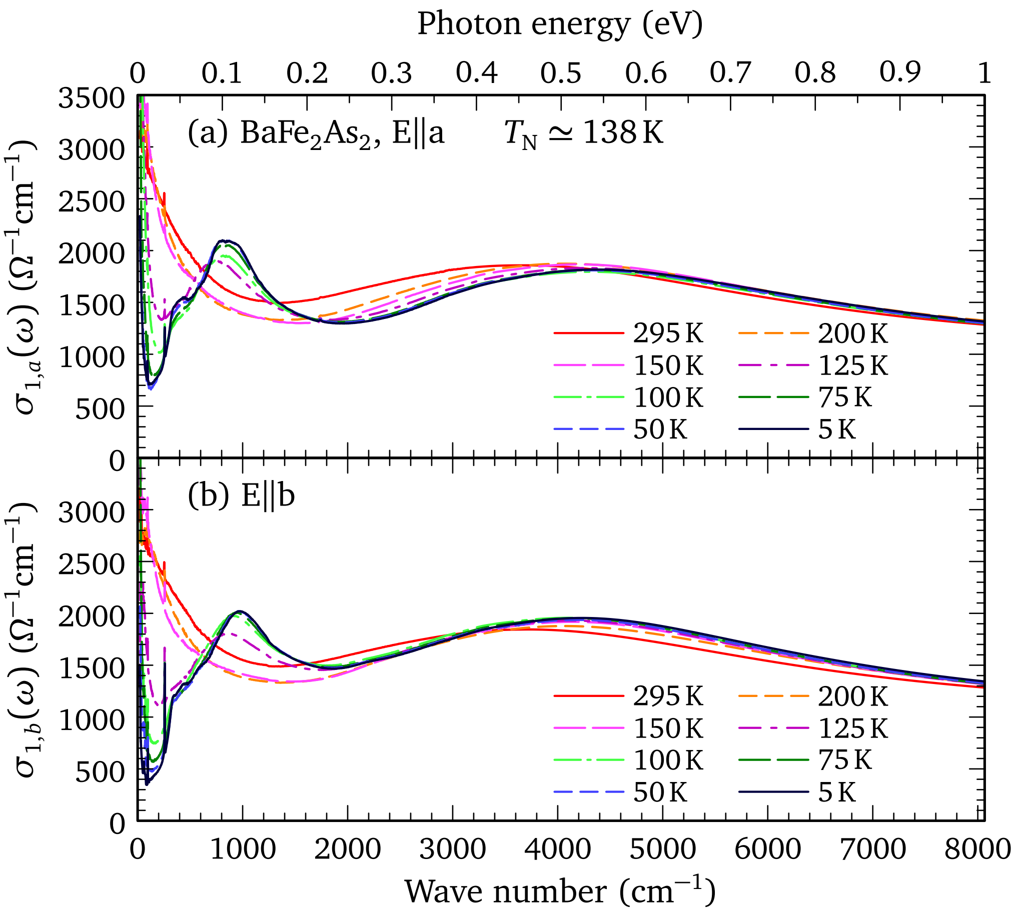


Figure S2. The temperature dependence of the real part of the optical conductivity versus frequency of a detwinned sample of $BaFe_2As_2$ for light polarized along the: (a) $a$ axis; (b) $b$ axis.

The differences in the optical conductivity in the mid-infrared region appear to be due to the anisotropic behavior of the free-carriers below $T_N$.

## VIBRATIONAL PROPERTIES

In addition to the temperature and polarization dependence of the reflectivity of $BaFe_2As_2$ in the far-infrared region that was measured with an instrumental resolution of 1.8 cm$^{-1}$, the reflectivity at $\sim$ 5 K was also measured with a resolution of 1.0 cm$^{-1}$; this measurement was performed with a thick silicon beam splitter which has a maximum resolution of $\sim$ 0.9 cm$^{-1}$. The improved resolution allows the $E_u \to B_{2u} + B_{3u}$ low-temperature splitting of the low-frequency $E_u$ mode in the orthorhombic phase to be clearly observed (detailed in the manuscript). The low-frequency modes are described quite well by symmetric Lorentzian oscillators. However, at low temperature the high-frequency modes show a slightly asymmetric profile. It is possible that coupling to either a spin or charge background may result in an asymmetric line shape. Accordingly, the infrared-active vibrations have been fit using a phenomenological complex dielectric function, $\tilde{\epsilon} = \epsilon_1 + i\epsilon_2$, for a Fano-shaped Lorentz oscillator [2, 3],

$$\tilde{\epsilon}(\omega) = \frac{\Omega_0^2}{\omega_0^2 - \omega^2 - i\gamma_0\omega}\left(1 + i\frac{\omega_q}{\omega}\right)^2 + \left(\frac{\Omega_0\omega_q}{\omega_0\omega}\right)^2, \tag{S1}$$

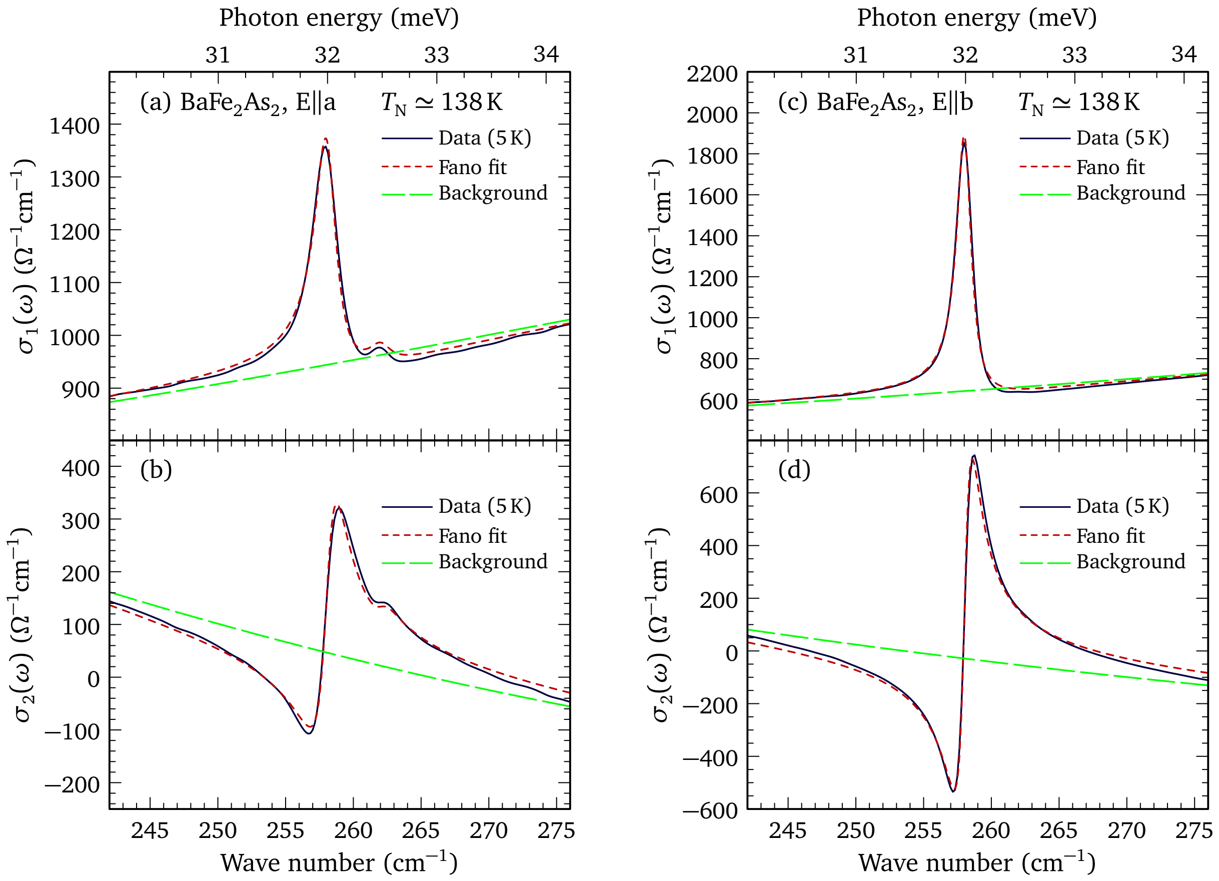


Figure S3. The fit of the Fano lineshape in Eq. (S1) in combination with the Drude-Lorentz model for the electronic continuum to the (a) real, and (b) imaginary part of the optical conductivity to the high-frequency $E_u$ mode in $BaFe_2As_2$ at $\sim 5$ K for light polarized along the $a$ axis; and to the (a) real, and (b) imaginary part of the optical conductivity for light polarized along the $b$ axis at $\sim 5$ K. The solid line indicates the data, the long-dashed line the electronic background, and the short-dashed line is the overall fit to the data.

where $\omega_0$, $\gamma_0$ and $\Omega_0$ are the position, width, and strength of the vibration, respectively, and the asymmetry is described by the dimensionless parameter $1/q^2 = (\omega_q/\omega_0)^2$; in the limit of $1/q^2 \to 0$, a symmetric Lorentzian oscillator is recovered. The complex conductivity is $\tilde{\sigma}(\omega) = \sigma_1 + i\sigma_2 = -2\pi i\omega[\tilde{\epsilon}(\omega) - \epsilon_\infty]/Z_0$ (in units of $\Omega^{-1}\text{cm}^{-1}$), where $\epsilon_\infty$ is the high-frequency contribution to the real part of the dielectric function, and $Z_0 \simeq 377\ \Omega$ is the impedance of free space.

The low-temperature fit to the real and imaginary parts of the optical conductivity of the high-frequency mode for light polarized along the $a$ axis is shown in Figs. S3(a) and S3(b), respectively; the fit reveals a strong oscillator at $\simeq 258$ cm$^{-1}$ which is attributed to the $B_{2u}$ mode normally active along the $b$ axis, but which is present here due to the fact that the sample is not completely detwinned. The higher resolution allows the very weak $B_{3u}$ mode at

Table I. The frequency ($\omega_i$), width ($\gamma_i$), strength ($\Omega_i$), and asymmetry parameter ($1/q_i$) for the fits to the Fano line shape in Eq. (S1) to the low- and high-frequency $B_{2u}$ and $B_{3u}$ vibrational modes in the orthorhombic phase of a detwinned single crystal of $BaFe_2As_2$ at 5 K.

| | E‖a | | | | E‖b | | | |
|---|---|---|---|---|---|---|---|---|
| mode | $\omega_i$ (cm$^{-1}$) | $\gamma_i$ (cm$^{-1}$) | $\Omega_i$ (cm$^{-1}$) | $1/q_i^2$ | $\omega_i$ (cm$^{-1}$) | $\gamma_i$ (cm$^{-1}$) | $\Omega_i$ (cm$^{-1}$) | $1/q_i^2$ |
| $B_{2u}(1)$ | 93.8 | 1.1 | 151 | $\sim 0$ | 95.3 | 1.0 | 85 | $\sim 0$ |
| $B_{3u}(1)$ | 96.5 | 1.1 | 106 | $\sim 0$ | 96.4 | 1.1 | 198 | $\sim 0$ |
| | | | | | | | | |
| $B_{2u}(2)$ | 258.1 | 1.9 | 222 | 0.034 | 258.1 | 1.4 | 313 | 0.011 |
| $B_{3u}(2)$ | 262.1 | 2.0 | 65 | 0.013 | – | – | – | – |

$\simeq$ 262 cm$^{-1}$ to be observed. The electronic background is described by the Drude-Lorentz terms described in the manuscript.

The fit to the real and imaginary parts of the optical conductivity at $\sim$ 5 K for light polarized along the $b$ axis is shown in Figs. S3(c) and S3(d), respectively, revealing a very strong $B_{2u}$ mode at $\simeq$ 258 cm$^{-1}$ with a weak asymmetry. Despite the fact that the sample is not completely detwinned, there is no sign of the weak $B_{3u}$ mode in this polarization. The results of the fits are summarized in Table I.

* homes@bnl.gov
† christoph.meingast@kit.edu
[1] M. Nakajima, T. Liang, S. Ishida, Y. Tomioka, K. Kihou, C. H. Lee, A. Iyo, H. Eisaki, T. Kakeshita, T. Ito, and S. Uchida, "Unprecedented anisotropic metallic state in undoped iron arsenide $BaFe_2As_2$ revealed by optical spectroscopy," PNAS **108**, 12238–12242 (2011).
[2] A. Damascelli, *Optical Spectroscopy of Quantum Spin Systems*, Ph.D. thesis, University of Groningen (1996), p. 21.
[3] A. Kuzmenko, Software RefFIT, Manual p. 64 (2014).
